# Supplementary material for: Dating and localizing an invasion from post-introduction data and a coupled reaction-diffusion-absorption model
Source: arXiv:1808.00868 ancillary file (2018-08-01)
Supplement: Supplementary file 1 [file ESM.pdf]

**Electronic Supplementary Material (EMS)**

# Dating and localizing an invasion from post-introduction data and a coupled reaction-diffusion-absorption model

C. Abboud[1], O. Bonnefon[1], E. Parent[2], and S. Soubeyrand[1]

[1]BioSP, INRA, 84914 Avignon, France

[2] AgroParisTech, UMR 518 Math. Info. Appli., Paris, France,

INRA, UMR 518 Math. Info. Appli., Paris, France

## S1 Numerical Equation Solving

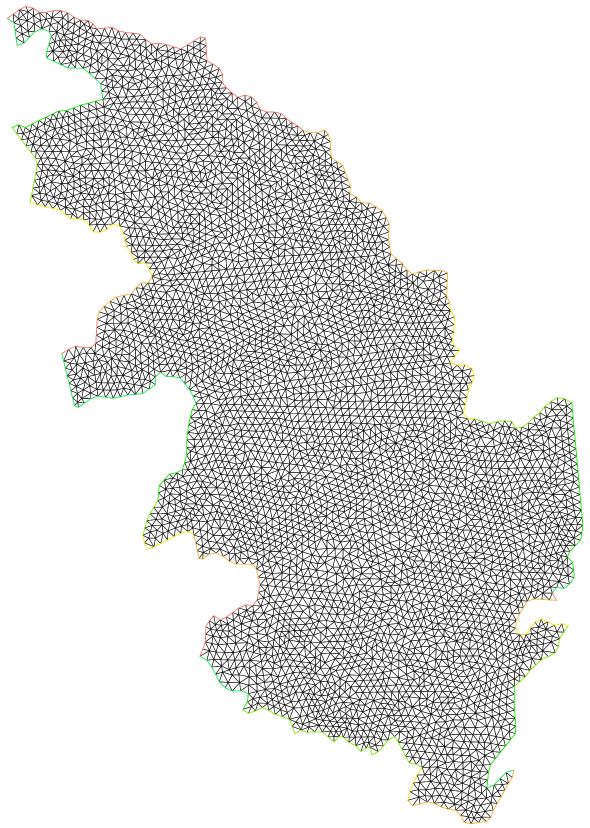

Figure S1: Mesh used for the Finite Element Method. This mesh contains 4791 nodes and 9141 triangles. The geometrical characteristics of this mesh were used to compute the accuracy of the simulator.

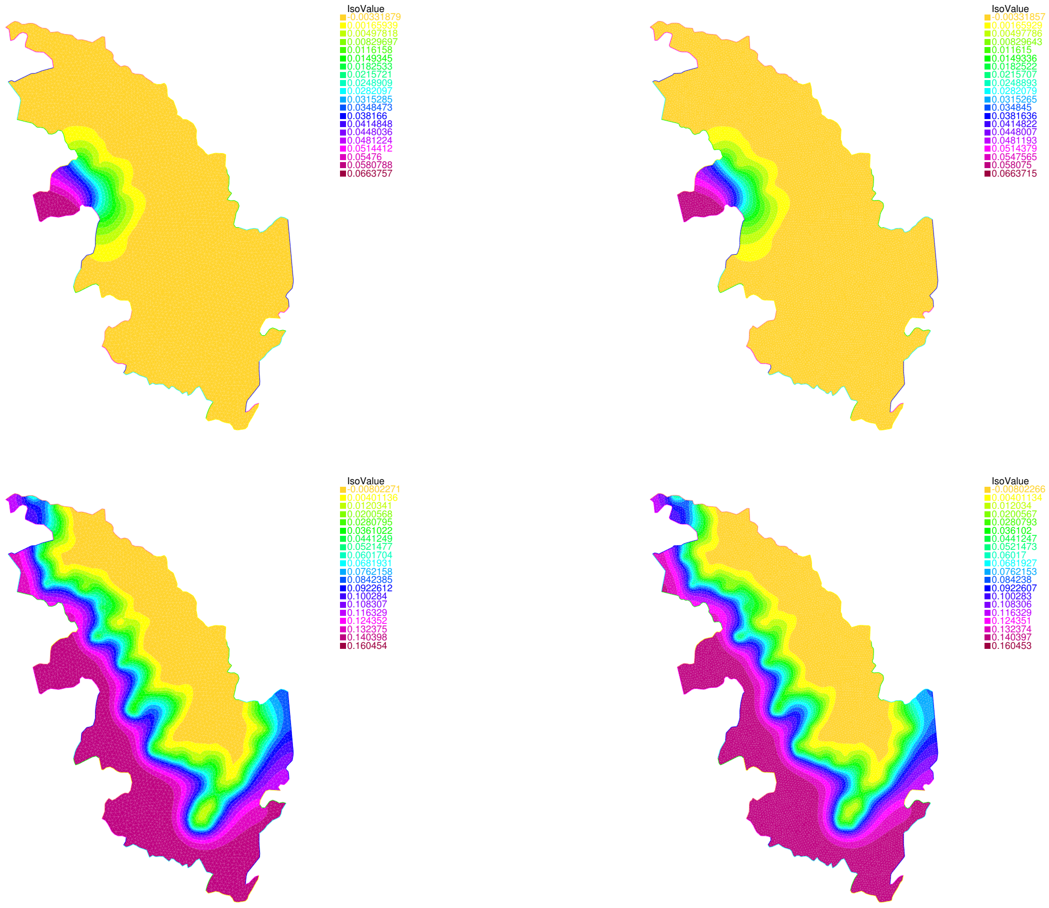


Figure S2: Probability of infection obtained at two different times and with two different meshes for the parameter vector corresponding to the posterior maximum. Top panels: 100 months after the introduction; Bottom panels: time of the last observation; Left panels: mesh composed of 4791 nodes; Right panel: finer mesh with 10703 nodes. Average difference between (a) and (b): $3e^{-5}$; Maximal difference: 0.002. Average difference between (c) and (d): $4e^{-5}$; Maximal difference: 0.02.

# S2 Local Brier Score

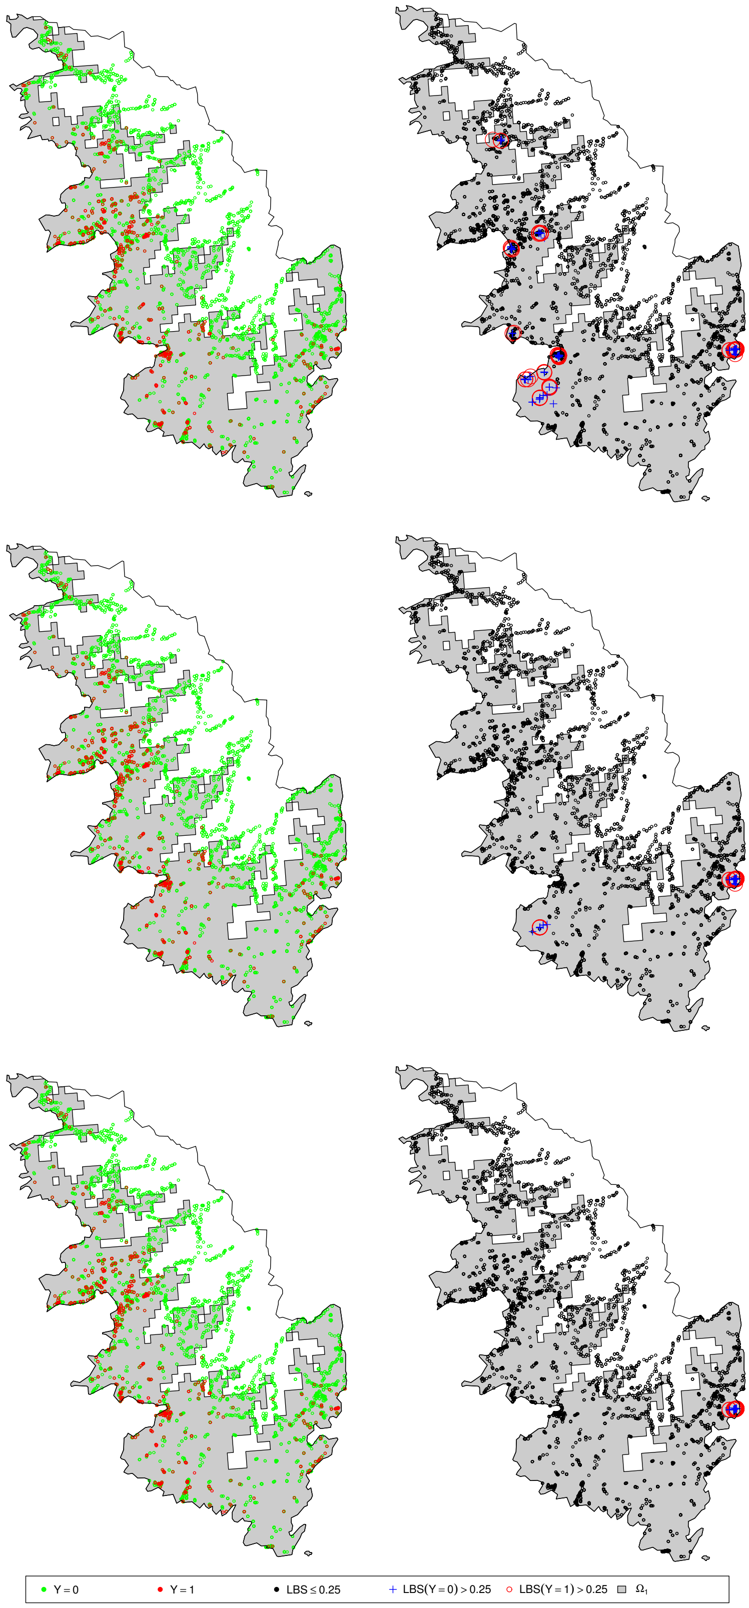


Figure S3: Locations where the LBS given in section 3.5.1 (main text) is larger than 0.25 with $k = 50$ (top), $k = 100$ (center), $k = 150$ (bottom). The gray surface gives the extent of $\Omega_1$.
